# Supplementary material for: Progressive Cluster Purification for Unsupervised Feature Learning
Source: arXiv:2007.02577 source file (2020-07-15)
Supplement: Supplementary file 1 [file appendix.tex]

\appendix
\section{Appendix}
\subsection{Dataset}
 We select IN-10, IN-50 and IN-100 from ILSVRC2012 dataset. For example, IN-100 includes: \\
n02869837, n01749939, n02488291, n02107142, n13037406, \\
n02091831, n04517823, n04589890, n03062245, n01773797, \\
n01735189, n07831146,  n07753275, n03085013, n04485082,\\
n02105505, n01983481, n02788148, n03530642, n04435653,\\
n02086910, n02859443, n13040303, n03594734, n02085620,\\
n02099849, n01558993, n04493381, n02109047, n04111531,\\
n02877765, n04429376, n02009229, n01978455, n02106550,\\
n01820546, n01692333, n07714571, n02974003, n02114855,\\
n03785016, n03764736, n03775546, n02087046, n07836838,\\
n04099969, n04592741, n03891251, n02701002, n03379051,\\
n02259212, n07715103, n03947888, n04026417, n02326432,\\
n03637318, n01980166, n02113799, n02086240, n03903868,\\
n02483362, n04127249, n02089973, n03017168, n02093428,\\
n02804414, n02396427, n04418357, n02172182, n01729322,\\
n02113978, n03787032, n02089867, n02119022, n03777754,\\
n04238763, n02231487, n03032252, n02138441, n02104029,\\
n03837869, n03494278, n04136333, n03794056, n03492542,\\
n02018207, n04067472, n03930630, n03584829, n02123045,\\
n04229816, n02100583, n03642806, n04336792, n03259280,\\
n02116738, n02108089, n03424325, n01855672, n02090622.\\
IN-10 and IN-50 include first 10 and 50 classess, respectively.
% \subsection{Experimental setup}

% \paragraph{Architectures} Within an exp.
